# Supplementary material for: Navigating Resource Conflicts: Co-opetition and Fairness
Source: arXiv:2311.04603 source file (2023-11-08)
Supplement: Supplementary file 1 [file Appendix_comp.tex]

\chapter{Proofs Related to Chapter~\ref{chap_comp}}

\label{chap_appendix_comp}

\textbf{Proof of Lemma \ref{lem_uni_LQ}: } Consider any partition $\P$. If $\P$ = ALC, then none of the players can deviate unilaterally, and hence configuration $(\P,{\bm \phi})$ with ${\bm \phi} = (\nu_{\{1\}},\cdots,\nu_{\{n\}})$ is stable. 

On the other hand, consider a partition $\P$ such that there exists at least one player $i$ in some coalition $C_j$ with $|C_j| \ge 2$. Say player $i$ deviates unilaterally to being alone. Then  under pessimistic anticipation rule, player $i$ on deviating obtains $\ulam_i$. Using Theorem \ref{Thm_WE}, \begin{equation}
   \nu_{C_j}^\P > \sum_{n \in C_j} \ulam_n.
   \label{eq_strict_coal_worth}
\end{equation}
Thus $(\P,{\bm \phi})$ is stable when each player $i$ gets strictly more than $\ulam_i$ and $\sum_{n \in C_j} \phi_n = \nu_{C_j}^\P$, which is possible from \eqref{eq_strict_coal_worth}. One such configuration is $(\P,{\bm \phi})$ where 
$$\phi_k = \ulam_k + \frac{1}{|C_j|}\left(\nu_{C_j}^\P - \sum_{n \in C_j} \ulam_n \right) \text{ for all } k \in C_j.$$
